# Supplementary material for: Mechanics-Informed Autoencoder Enables Automated Detection and Localization of Unforeseen Structural Damage
Source: arXiv:2402.15492 source file (2024-07-18)
Supplement: Supplementary file 1 [file Supplementary.pdf]

# Supplementary Information for:

## Mechanics-Informed Autoencoder Enables Automated Detection and Localization of Unforeseen Structural Damage

### Supplementary Note 1: Crack localization for more cases in FEM simulation

In Fig. 2 of the article, the rectangular-shaped crack is determined by 5 variables  $C_x$ ,  $C_y$ ,  $l$ ,  $w$ , and  $\alpha$ , representing the crack center horizontal coordinates, center vertical coordinates, length, width, and the crack angle, respectively. However, only a typical crack case is evaluated, where the crack location and orientation are kept constant.

We conducted a comprehensive assessment of different crack scenarios with varying crack properties through numerical experiments. In multiple testing cases, we introduced random variations in parameters  $C_x$ ,  $C_y$ ,  $w$ , and  $\alpha$ , simulating the propagation of cracks from an initial length of 8mm to 40mm. The model's performance for crack localization is shown in Supplementary Fig. 1. The mechanics' knowledge enables strong sensor correlations and amplifies the reconstruction errors during the evaluation. Therefore, the localization contours display discrepancies much earlier than the standard autoencoder method.

### Supplementary Note 2: The underlying mechanism for early damage detection and localization

**Early damage detection mechanism** The incorporation of mechanics' relations in Mechanics-Informed Autoencoder (MIAE) significantly improves the damage detection rate through two key mechanisms. Firstly, the training of MIAE reduces overall training reconstruction errors, leading to a more concentrated error distribution on the left side of Supplementary Fig. 2. Secondly, MIAE substantially increases the magnitude of testing reconstruction errors from damaged structures as depicted on the right side left side

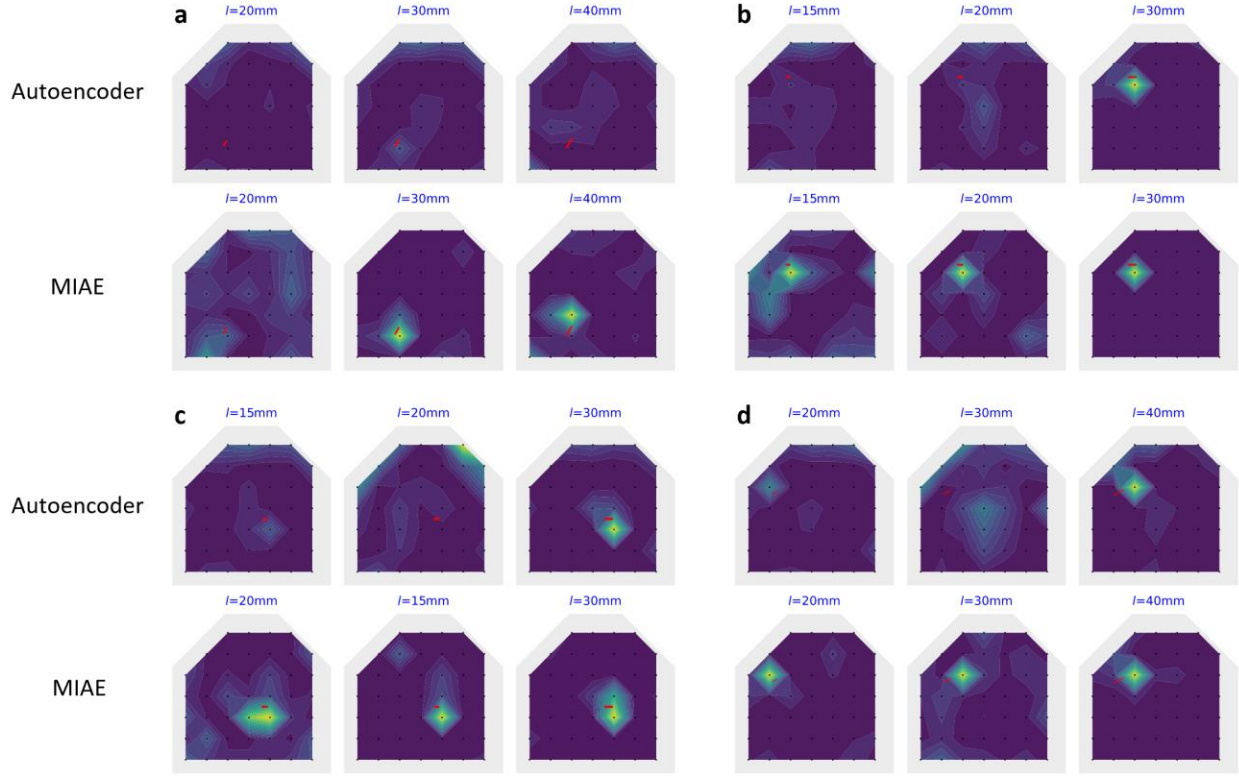

**Supplementary Figure 1:** Damage localization at a variety of crack scenarios. The proposed MIAE (second row) can localize cracks much earlier than the standard autoencoder (first row). **a**, **b**, **c**, and **d** show four different crack cases within the plate structure. In each case, the angle, width, and center point of the crack have a unique combination.

of Supplementary Fig. 2. Consequently, testing reconstruction errors resulting from minor damage conditions in the early stages of damage progression become clearly distinguishable from training reconstruction errors. This heightened distinction contributes to a higher detection accuracy compared to the conventional autoencoder method. As damage further propagates, both MIAE and the autoencoder method are expected to demonstrate similar detection performance. This similarity arises as the reconstruction error distributions shift to the right, becoming distinguishable from the undamaged distribution in both methods.

**Early damage localization mechanism** MIAE improves the localization performance by greatly amplifying the damage scores  $p$ . The underlying mechanism for early localization parallels the detection

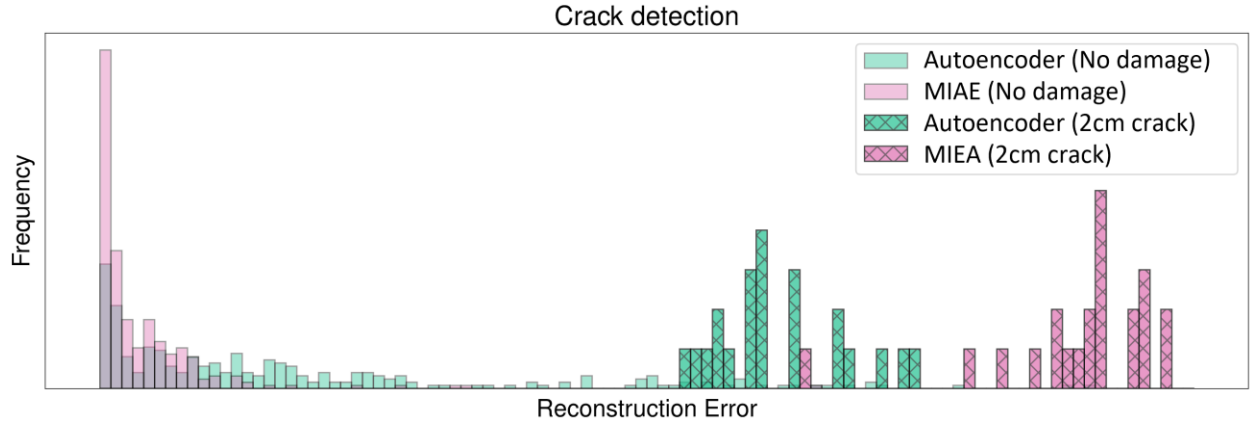

**Supplementary Figure 2.** Demonstration of the underlying mechanism for MIAE. Compared to the autoencoder method, MIAE learns a more effective undamaged reference, with lower distribution errors and less variations. Furthermore, MIAE exhibits significantly larger reconstruction errors from damaged structural conditions.

process described earlier. In MIAE, the ratio of norm errors from training to testing is much larger than in a standard autoencoder. This heightened ratio increases sensitivity and leads to larger  $p$  values, ultimately creating contours with sharper contrast in damaged areas compared to undamaged regions.

To illustrate the improvement in contour values, we present the experimental results of MIAE in Supplementary Fig. 3a-c, covering the crack scenario and the initial and final stages of the boundary condition variation. Specifically, the  $\mu$  and  $\sigma$  feature contours for the crack scenario are displayed separately. Both methods yield visually similar contours among all cases, yet there is a notable difference in contour values. The contours values derived from MIAE (second row) are greater than the values from a standard autoencoder (first row). Additionally, MIAE demonstrates higher sensitivity in the scenario of boundary condition variation. Supplementary Fig. 3d illustrates the progression of the relative magnitude changes of the peak value from the  $\mu$  feature. MIAE displays a notably faster increase rate during damage progression, initiating from an initial value (72,000) 22 times greater than the autoencoder's value (3,150) shown from Supplementary Fig. 3b. In summary, both experiments demonstrate that MIAE significantly amplifies testing errors from the damaged structure, effectively isolating samples from damaged structures and thus, enhance the overall detection accuracy.

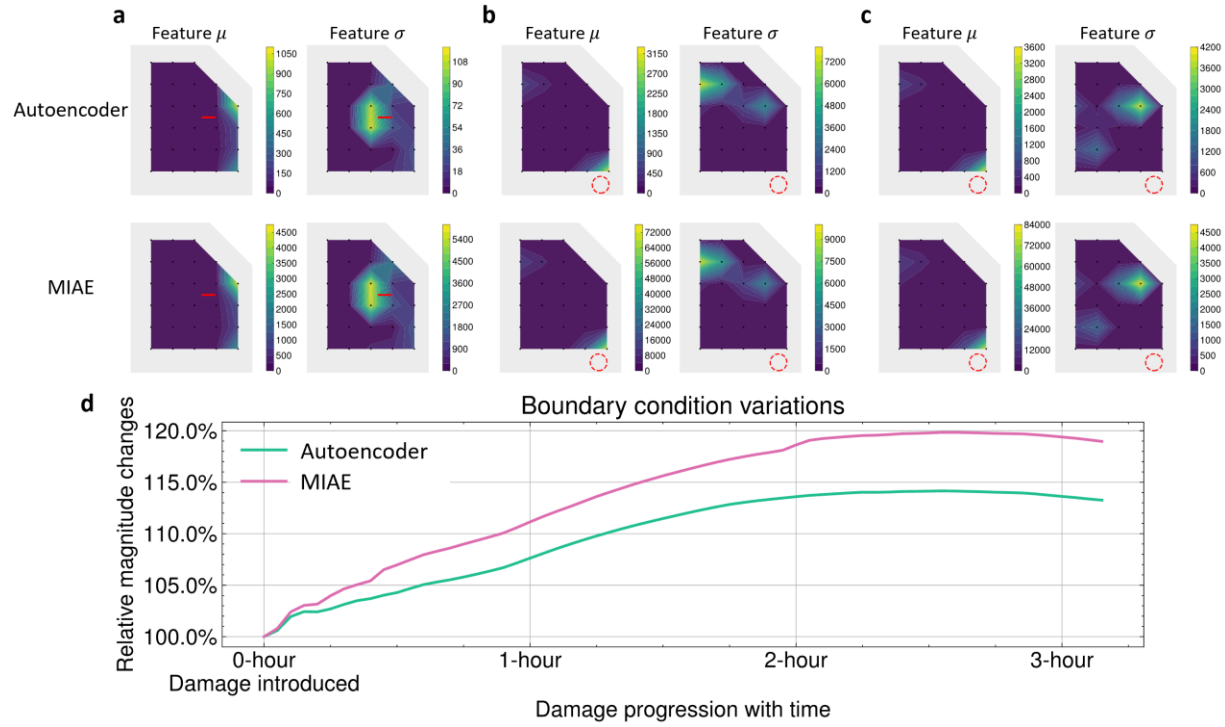

**Supplementary Figure 3.** Analysis of  $\mu$  and  $\sigma$  feature contours in MIAE and autoencoder. MIAE greatly amplifies the peak magnitude from the feature type most associated with the type of damage. In detail,  $\mu$  is more related to boundary condition variations, and  $\sigma$  is more indicative of crack damages. **a.** The two feature contours for the crack scenario. **b.** The two feature contours for the initial loading stage of the boundary condition variation scenario. **c.** The two feature contours for the late loading stage of the boundary condition variation scenario. **d.** The relative changes of peak magnitude with damage progression.

### Supplementary Note 3: Damage differentiation

MIAE exhibits the ability to differentiate between crack damages and boundary condition variations by analyzing the  $\mu$  and  $\sigma$  contours. Specifically,  $\sigma$  is more closely associated with crack damage. This is evident in the lower row of Supplementary Fig. 3a, where the peak value in the  $\sigma$  feature contour is substantial and has a significant influence on the damage score  $p$ . In contrast,  $\mu$  is more closely related to boundary condition variations, as indicated by the corresponding peak values in Supplementary Fig. 3b-c, which are larger than those from the  $\sigma$  feature contour. In Supplementary Fig. 4, a representative case with three different crack lengths (2cm, 3cm, and 4cm from left to right) from the numerical simulation of cracks is displayed, with the dominance observed from the  $\sigma$  feature contour (second row). In Supplementary Fig. 4a for the autoencoder method, both types of contours appear visually similar, but the  $\mu$  feature contours

exhibit very low magnitudes compared to the undamaged reference (a maximum magnitude of 1). In contrast,  $\sigma$  feature contours display significantly larger magnitudes, providing clear differentiation from the undamaged reference. Moving to Supplementary Fig. 4b, the proposed MIAE correctly localizes all presented crack lengths. However, similar to the autoencoder results,  $\sigma$  feature contours exhibit relatively larger magnitudes when compared to  $\mu$  feature contours. This observation demonstrates the closer association of the  $\sigma$  feature with cracks, and further helps differentiate cracks and boundary condition variations.

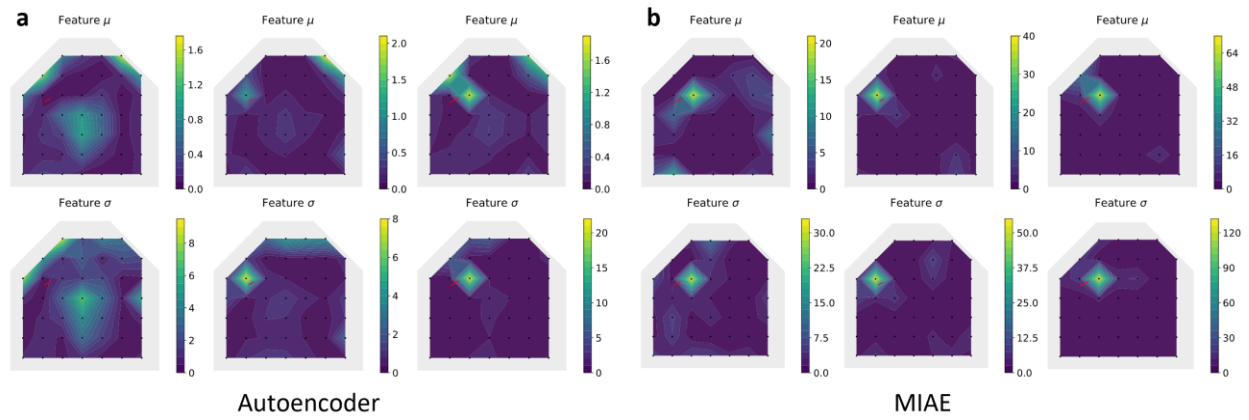

**Supplementary Figure 4.**  $\mu$  and  $\sigma$  feature contours for crack localization. **a.**  $\mu$  and  $\sigma$  feature contours for different crack lengths using autoencoder. The crack lengths, from left to right, are 2cm, 3cm, and 4cm. The autoencoder fails to localize the crack at 2cm. **b.**  $\mu$  and  $\sigma$  feature contours for different crack lengths using MIAE. The  $\sigma$  features presented have notably higher peak values, indicating a stronger association with cracks.

#### Supplementary Note 4: Machine learning methods comparison in structural engineering

In the field of structural engineering, Physical-Informed Neural Network (PINN) <sup>[1-2]</sup> and Graph Neural Network (GNN) <sup>[3-5]</sup> are widely used deep learning methods that can potentially be employed for the task we consider in this paper. However, these approaches largely focus on forward and inverse problems instead of SHM. Existing GNN for forward structural analysis primarily focuses on trusses, which usually involve static analysis of a limited number of nodal elements and well-defined boundary conditions. Other GNNs may integrate with LSTMs for forecasting responses like strain values <sup>[6]</sup>, enabling the detection of structural anomalies by identifying deviations from expected behavior under operational conditions. In

addition, it is essential to note that graph convolutional networks (GCNs) <sup>[7]</sup> are also popularly used for damage detection. However, these methods are supervised, making it difficult to generalize across various structures, as labeled damage data may be challenging to obtain during the training stage. On the other hand, while PINN models are frequently used for modeling structural responses and have been extended to dynamic analysis <sup>[8]</sup>, their application in SHM is challenging. Real-world structures often feature unknown constraints and lack detailed information about loading conditions. PINNs generally require extensive spatial measurements, which may not be feasible due to the impracticality of installing numerous sensors. These limitations hinder the effective application of PINN models in practical SHM contexts.

The following Table is a supplement of the introduction. It is acknowledged that many different methods are utilized for structural engineering. However, those popular methods require additional information that may be difficult to obtain in the normal SHM setting.

**Supplementary Table 1:** ML method comparison for structural engineering

| Methods                                       | Require known PDEs | Require BCs & forces data | Supervised (labels) | Require response data |
|-----------------------------------------------|--------------------|---------------------------|---------------------|-----------------------|
| PINN <sup>[1-2]</sup>                         | √                  | √                         | √                   | √                     |
| GNN <sup>[3-5]</sup>                          |                    | ~                         | √                   | √                     |
| GCN <sup>[7]</sup>                            |                    |                           | √                   | √                     |
| <b>MIDAS</b>                                  |                    |                           |                     | √                     |
| ~: vary depending on the specific application |                    |                           |                     |                       |

[1] Raissi, Maziar, and George Em Karniadakis. "Hidden physics models: Machine learning of nonlinear partial differential equations." *Journal of Computational Physics* 357 (2018): 125-141.

[2] Raissi, Maziar, Paris Perdikaris, and George E. Karniadakis. "Physics-informed neural networks: A deep learning framework for solving forward and inverse problems involving nonlinear partial differential equations." *Journal of Computational physics* 378 (2019): 686-707.

[3] Parisi, Fabio, et al. "On the use of mechanics-informed models to structural engineering systems: Application of graph neural networks for structural analysis." *Structures*. Vol. 59. Elsevier, 2024.

[4] Song, Ling-Han, et al. "Elastic structural analysis based on graph neural network without labeled data." *Computer-Aided Civil and Infrastructure Engineering* 38.10 (2023): 1307-1323.

[5] Chou, Yuan-Tung, et al. "StructGNN: An efficient graph neural network framework for static structural analysis." *Computers & Structures* 299 (2024): 107385.

- [6] Bloemheugel, Stefan, Jurgen van den Hoogen, and Martin Atzmueller. "A computational framework for modeling complex sensor network data using graph signal processing and graph neural networks in structural health monitoring." *Applied Network Science* 6.1 (2021): 97.
- [7] Zhan, Pengming, et al. "A Novel Structural Damage Detection Method via Multisensor Spatial–Temporal Graph-Based Features and Deep Graph Convolutional Network." *IEEE Transactions on Instrumentation and Measurement* 72 (2023): 1-14.
- [8] Bolandi, Hamed, et al. "Physics informed neural network for dynamic stress prediction." *Applied Intelligence* 53.22 (2023): 26313-26328.

### Supplementary Note 5: Generation of traffic loading

We assume that random structural loading, or traffic loading can be generated by the Fourier series. With randomized parameters, the model mimics the complex interplay between predictable traffic patterns (e.g., daily rush hours) and inherent randomness (e.g., vehicle mix, cargo fluctuations). This could effectively simulate the varying amplitude, frequency, and direction of traffic loads on a structure. The loads, discretized in the x or y components, consist of combinations of randomly generated sine and cosine functions:

$$load_m(x/y \text{ direction}) = \begin{cases} A_0 + \sum_{n=1}^{20} [A_n \cos \omega(t - t_0) + B_n \sin \omega(t - t_0)] & \text{for } t \geq t_0, \\ A_0 & \text{for } t < t_0, \end{cases}$$

where coefficients  $A_0, \omega, A_n, B_n, t_0$  are randomly chosen based on distributions.  $A_0, A_n$  and  $B_n$  follow a normal distribution of  $N(0,1)$ .  $\omega$  follows a normal distribution of  $N(4\pi, \frac{3}{2}\pi)$ .  $t_0$  follows a random distribution between 0 and 1. The subscript  $m$  is 5, indicating that 5 loadings are applied to the same location of the structure in the same direction ( $x$  or  $y$ ). This further increases the complexity of random loading. Thus, the total force in one direction is:

$$F_{x/y} = \text{amplitude} * \sum_{m=1}^5 load_m(x/y \text{ direction})$$

The amplitude is calculated as pressure multiplying the loading length and plate thickness,  $\text{amplitude} = 1,000,000 \times 0.2 \times 0.012 = 2,400N = 2.4kN$ . As each load component  $\text{load}_m$  is randomly generated, the maximum load magnitude in total is expected to be around  $2,000kN$ . Regarding the time variation, the timestep is set to  $0.025s$  for the simulation and  $0.1s$  for the experiment to ensure accurate loading is applied by the machine in the real experiment.

### Supplementary Note 6: Sensor placement with fewer sensors

In the numerical simulation of the gusset plate, the sensors were strategically selected to ensure full coverage of the plate. In detail, we performed such selection 6 times for different number of sensors (4, 6, and 8 sensors). The corresponding sensor selections are displayed in Supplementary Fig. 5.

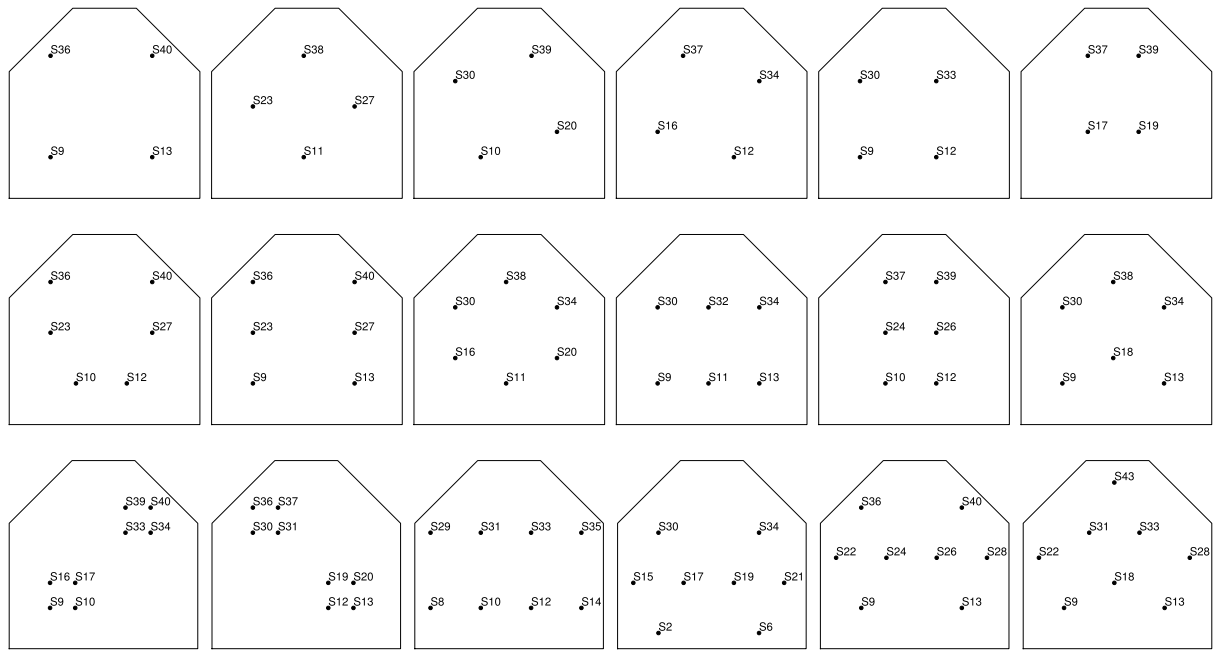

**Supplementary Figure 5.** Sensor placements for different number of sensors. The first, second, and third rows represent the sensor selection with 4, 6, and 8 available sensors.
